# Supplementary material for: Nanoscale magnetometry of a synthetic three-dimensional spin texture
Source: arXiv:2512.10476 source file (2026-03-13)
Supplement: Supplementary file 1 [file Supp_Info.pdf]

# Supplementary information: Nanoscale magnetometry of a synthetic three-dimensional spin texture

Ricardo Javier Peña Román,<sup>\*,†,‡,¶</sup> Sandip Maity,<sup>†,‡</sup> Fabian Samad,<sup>§,||</sup> Dinesh  
Pinto,<sup>†,⊥</sup> Simon Josephy,<sup>#</sup> Andrea Morales,<sup>#</sup> Attila Kákay,<sup>§</sup> Klaus Kern,<sup>†,⊥</sup> Olav  
Hellwig,<sup>§,||</sup> and Aparajita Singha<sup>\*,†,‡,¶</sup>

<sup>†</sup>*Max Planck Institute for Solid State Research, 70569 Stuttgart, Germany*

<sup>‡</sup>*Institute of Solid State and Materials Physics, Dresden University of Technology, 01069  
Dresden, Germany*

<sup>¶</sup>*Würzburg-Dresden Cluster of Excellence ct.qmat, 01069 Dresden, Germany*

<sup>§</sup>*Institute of Ion Beam Physics and Materials Research, Helmholtz-Zentrum  
Dresden-Rossendorf, 01328 Dresden, Germany*

<sup>||</sup>*Institute of Physics, Chemnitz University of Technology, 09107 Chemnitz, Germany*

<sup>⊥</sup>*Institute de Physique, Ecole Polytechnique Fédérale de Lausanne, CH-1015 Lausanne,  
Switzerland*

<sup>#</sup>*QZabre AG, 8050 Zurich, Switzerland*

E-mail: ricardo.pena\_roman@tu-dresden.de; aparajita.singha@tu-dresden.de

## Section 1: Characterization of the NV-diamond probes

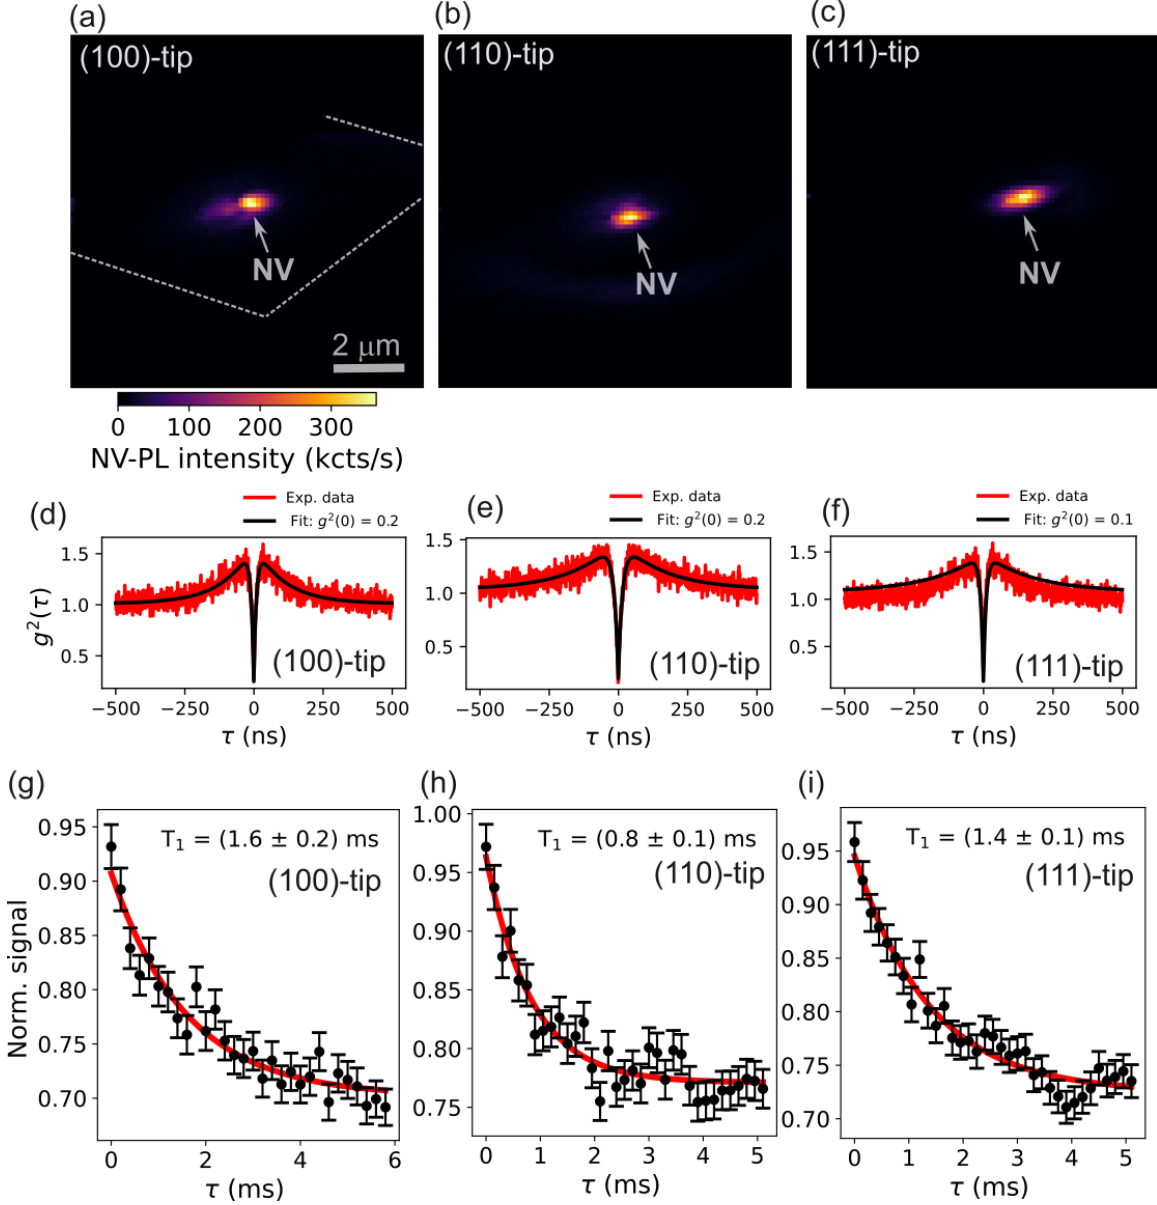

Figure S1: **Pre-characterization of commercial NV-probes.** (a)-(c) confocal images, (d)-(f) photon autocorrelation and (g)-(i)  $T_1$  measurements on (100), (110) and (111) NV-probes before approaching the sample. Green laser (515 nm) power of 130-300  $\mu\text{W}$ .

We used commercial scanning tips (Qzabre, Q6-Q7) with (100)-, (110)-, and (111)-oriented diamond crystals. Before approaching the sample to the tip and scanning, all tips are pre-characterized by confocal imaging, photon autocorrelation, and  $T_1$  measurements. Figures S1(a)-(c) show confocal images acquired with a green 515 nm laser using excitation power

of 130-300  $\mu\text{W}$ . Most of the light comes from the NV center, which appears as a bright spot with a signal above 300 kcts/s. The signal from the diamond base plate is weaker and not visible in the image. For reference, it is indicated by the white dashed line around the bright spot in panel (a). Figures S1(d)-(f) show the respective photon autocorrelation,  $g^2(\tau)$ , measurements where  $g^2(0) < 0.5$  confirms that there is a single NV defect in every tip. Additionally, Figures S1(g)-(i) show  $T_1$  measurements acquired using the pulse sequence described in the main text. The results indicate that these commercial tips with a nominal implantation depth of 10 nm exhibit longitudinal spin relaxation times of 0.8-1.4 ms. These  $T_1$  data are plotted in Figure 5(c) of the main text.

## Section 2: Calibration of the NV-sample distance

For quantitative measurements and comparison of data acquired with different scanning probes, it is essential to characterize the sensor-sample distance and the orientation of the single NV-spin. We used the conventional method described in the reference,<sup>1</sup> in which the stray field produced at the edges of a thin FM wire is corrected considering the topography profile and fitted by an analytical expression. As illustrated in Figure S2(a), for an FM wire along the y-axis, with thickness  $t$ , width  $W$ , and left and right edges at the positions  $x_L$  and  $x_R$ , respectively, the field at the distance  $d \gg t$  and position  $x$  is given by:

$$\begin{aligned}
\vec{B}^{wire}(x, 0, d) &= \vec{B}^{edge}(x - x_L, 0, d) + \vec{B}^{edge}(x - x_R, 0, d) \\
&= \frac{\mu_0 I_s}{2\pi} W \left[ d \left( \frac{w + 2(x_L - x)}{[(x - x_L)^2 + d^2][(x - x_R)^2 + d^2]} \right) \hat{e}_x + \left( \frac{x^2 + xw - 2xx_R + x_L x_R - wd^2}{[(x - x_L)^2 + d^2][(x - x_R)^2 + d^2]} \right) \hat{e}_z \right] \\
&= B_x^{wire}(x, 0, d) \hat{e}_x + B_z^{wire}(x, 0, d) \hat{e}_z
\end{aligned} \tag{1}$$

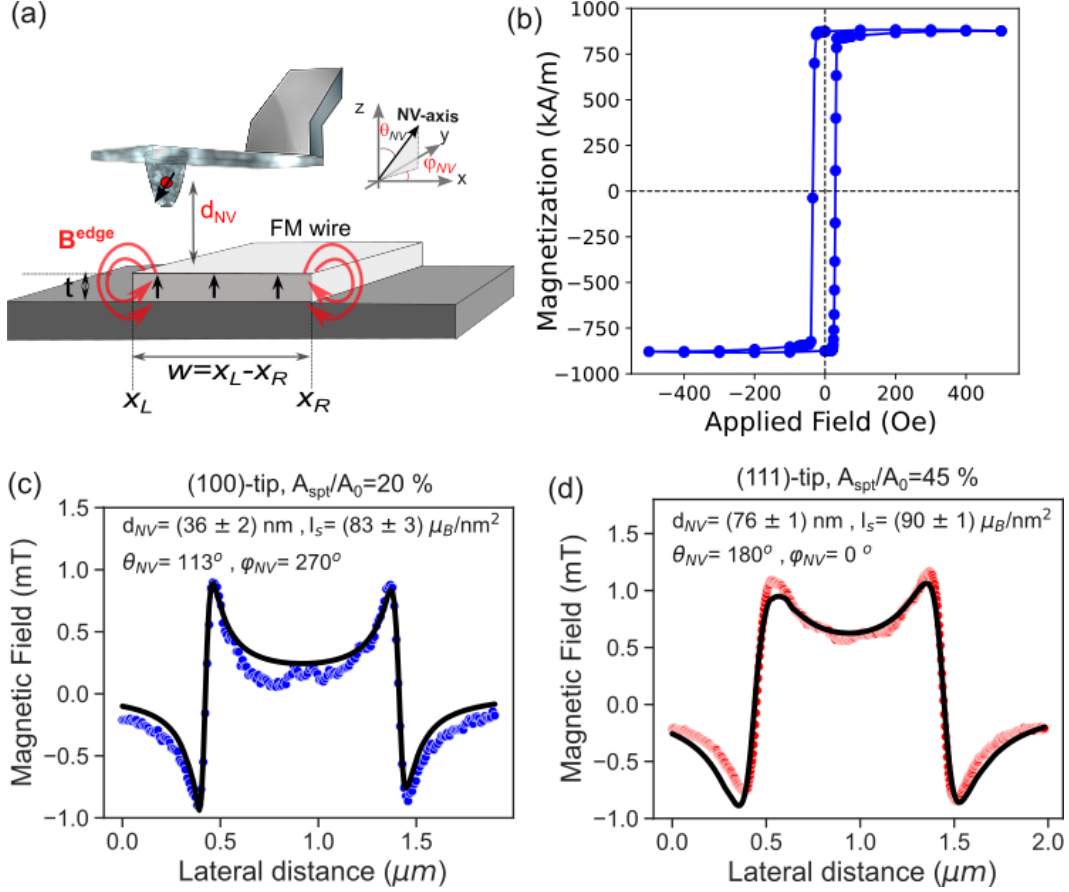

Figure S2: **Calibration sample and determination of the NV-sample distance.** (a) Schematic of the scanning probe and the stray field of a thin FM wire. We assume the wire parallel to the  $y$ -axis, and with magnetic thickness  $t \approx 1 \text{ nm}$ . The distance  $d_{NV}$  is determined from the sample surface and along the  $z$ -axis. The angles  $(\theta_{NV}, \varphi_{NV})$  determine the orientation of the NV-axis in the laboratory frame. (b) out-of-plane hysteresis curve of the calibration sample. (c) Fitting of the stray field profile measured across the wire with the (100)-NV tip and (d) with the (111)-NV tip. The fits are shown in solid black curves and the results as inset.

where  $I_s = M_s t$ , is the surface density of magnetic moments with  $M_s$  the saturation magnetization. The field sensed by the NV center is given by the projection of  $\vec{B}^{wire}(x, 0, d)$  along the NV-axis defined by the unit vector  $\hat{e}_{NV} = \cos \varphi_{NV} \sin \theta_{NV} \hat{e}_x + \sin \varphi_{NV} \sin \theta_{NV} \hat{e}_y + \cos \theta_{NV} \hat{e}_z$ , with the angles  $\varphi_{NV} \in [0^\circ, 360^\circ]$  and  $\theta_{NV} \in [0^\circ, 180^\circ]$ . Therefore, the field measured by the scanning-NV tip is:

$$B_{NV}(x, 0, d + \delta d) = B_x^{wire}(x, 0, d + \delta d) \cos \varphi_{NV} \sin \theta_{NV} + B_z^{wire}(x, 0, d + \delta d) \cos \theta_{NV} \quad (2)$$

The substitution  $d \rightarrow d + \delta d$  is introduced to include topography variations and measure the sensor-sample distance from the wire surface (topography correction).

We use as a calibration sample a FM wire of Ta/Pt/Co(0.6nm)/Pt deposited on a SiO<sub>2</sub>/Si substrate. The width of the wire is around 1  $\mu\text{m}$ , and the magnetic thickness is considered to be  $t \approx 1$  nm (0.6 nm (Co) + 2\*0.2 nm (Pt)). We assume 0.2 nm of Pt on both sides of the Co layer to contribute to the magnetic moment. Note that this value is not critical since  $I_s = M_s t$  is the relevant parameter and not  $M_s$  and  $t$  separately. The OOP hysteresis curve of the calibration sample is shown in Figure S2(b), from which we obtain an OOP saturation magnetization  $M_s = (884 \pm 88)$  kA/m. From here, we calculate  $I_s = (95 \pm 10)$   $\mu_B/\text{nm}^2$ . Stray field profiles measured across the FM wire with (100)- and (111)-NV probes are shown in Figure S2(c) and (d), respectively. The profiles are fitted using the expression in equation (2), and the results are presented as insets in the figures. We performed scanning using the amplitude modulation mode. The profile acquired with the (100)-probe was recorded using an amplitude setpoint ( $A_{stp}$ ) of 20% of the amplitude of the scanning tip in free space ( $A_0$ ). For calibration with a (111) probe the amplitude setpoint was set to  $A_{stp}/A_0 = 45\%$ , for which we obtain a higher NV-sample distance. The values for  $I_s$  obtained from the fitting are in good agreement with the experimental value. All the images recorded on the multilayered SAFs were acquired with similar scanning parameters to the calibration sample. Therefore, we expect the NV-sample distance to be in the range of 36-76 nm.

### **Section 3: Saturation magnetization and MFM images**

Figure S3(a) shows the OOP hysteresis curve measured at 300 K on the multilayered SAFs described in the main text. As represented in the figure, we observed four discrete steps in the loop, corresponding to the magnetic reversal of each of the FM blocks. The absolute total saturation magnetization is  $M_s = (833 \pm 83)$  kA/m, for configurations with a full magnetization pointing up/down. Figure S3(b) shows a large area MFM image, after saturation

with an IP field. The magnetic texture consists of large AF domains with periodic contrast along the FM stripes at the AF domain boundaries. A high-resolution MFM image is shown in Figure S3(c). Figure S3(d) shows profiles taken across and along a FM stripe. We estimate a FM stripe width of around 100 nm and a local periodicity of the contrast of 300 nm. In agreement with the observations by Hellwig *et al.*,<sup>2</sup> the non-zero integrated area of the profiles across the stripe demonstrate FM order.

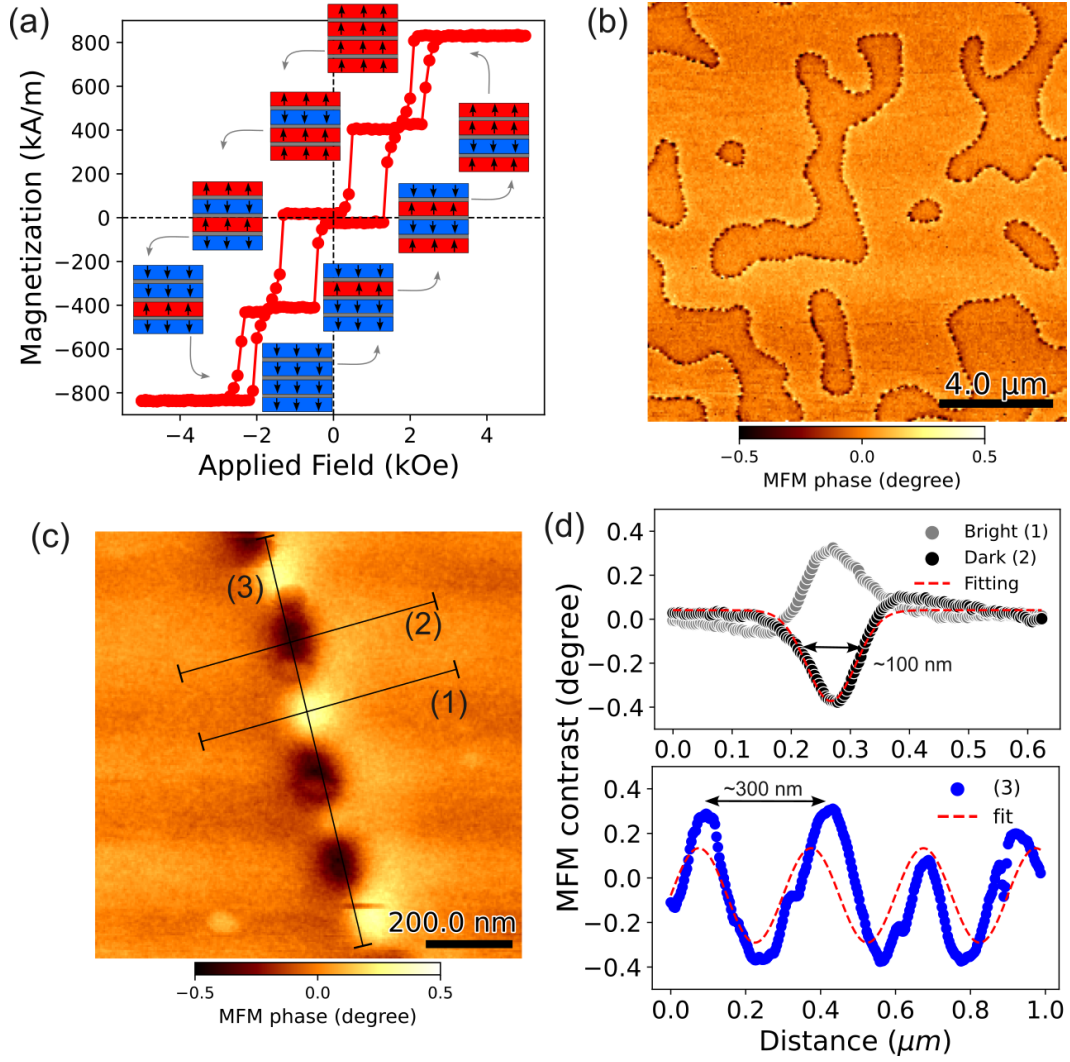

Figure S3: **Hysteresis curve and FM DW profiles.** (a) Out-of-plane hysteresis loop. (b) large area MFM image, 15 μm x 15 μm. (c) High resolution MFM image (1 μm x 1 μm) of the periodic contrast along the FM stripe at the AF domain boundary. (d) MFM profiles across and along the FM stripe. The FM stripe width and periodicity are estimated by fitting the profiles to a gaussian and sinusoidal function, respectively.

## Section 4: Additional ODMR measurements with the (100)-NV probe

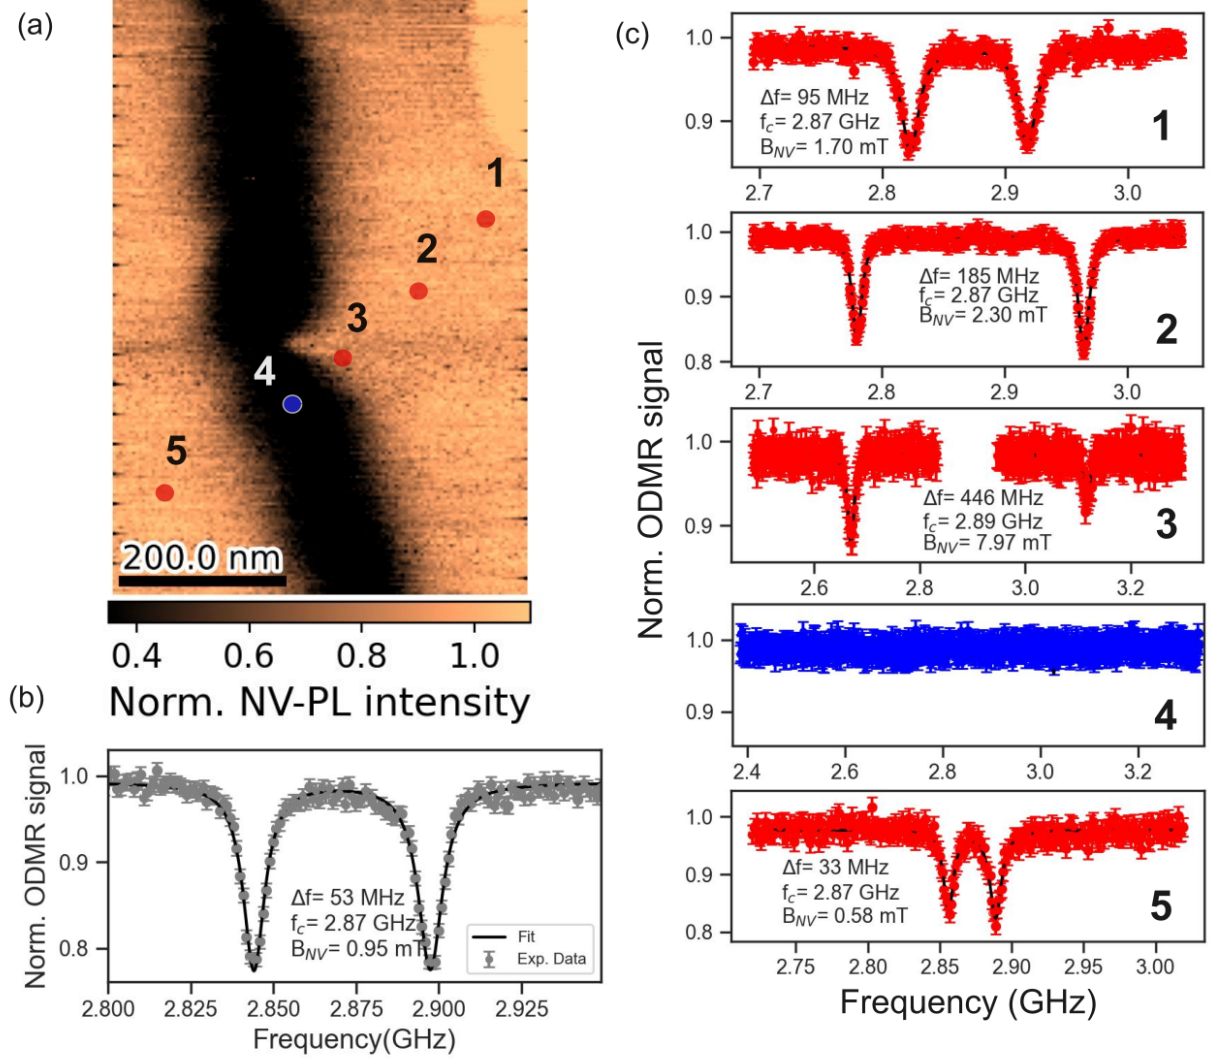

Figure S4: **Local ODMR measurements.** (a) NV-PL quenching map. (b) ODMR spectrum of the tip before approaching the sample. (c) ODMR spectra measured locally after approaching the sample and positioning the tip on the locations indicated in (a). The inset parameters in every plot correspond to the splitting ( $\Delta f$ ), the central frequency ( $f_c$ ), and the field sensed by the NV-center ( $B_{NV}$ ).

In Figure S4, we present ODMR measurements in addition to those shown in Figure 2 of the main text. In Figure S4(a), a high-resolution NV-PL quenching image is shown, recorded without applying any off-axis field to the NV sensor. In Figure S4(b) we observe

the ODMR spectrum of the tip before approaching the sample. The spectrum was acquired after turning off the electromagnet used to apply the external field. There is still a remnant external field that can be sensed by the NV, which gives rise to the initial splitting observed in the spectrum. Figure S4(c) shows ODMR spectra measured locally across the FM stripe between AF domains and at the positions 1-5 indicated in Figure S4(a). Close to the FM stripe, at position 3, the Zeeman shift is not symmetric with respect to  $f_0$ ; the central frequency is shifted from 2.87 GHz to 2.89 GHz. As discussed in the main text, it is an indication of spin-mixing induced by off-axis field components on the FM stripe. For some tip locations, the field is too strong, and it is not possible to see any splitting within the measured frequency range, as in the case of the spectrum measured at location 4.

## Section 5: NV-PL quenching and MFM-like contrast

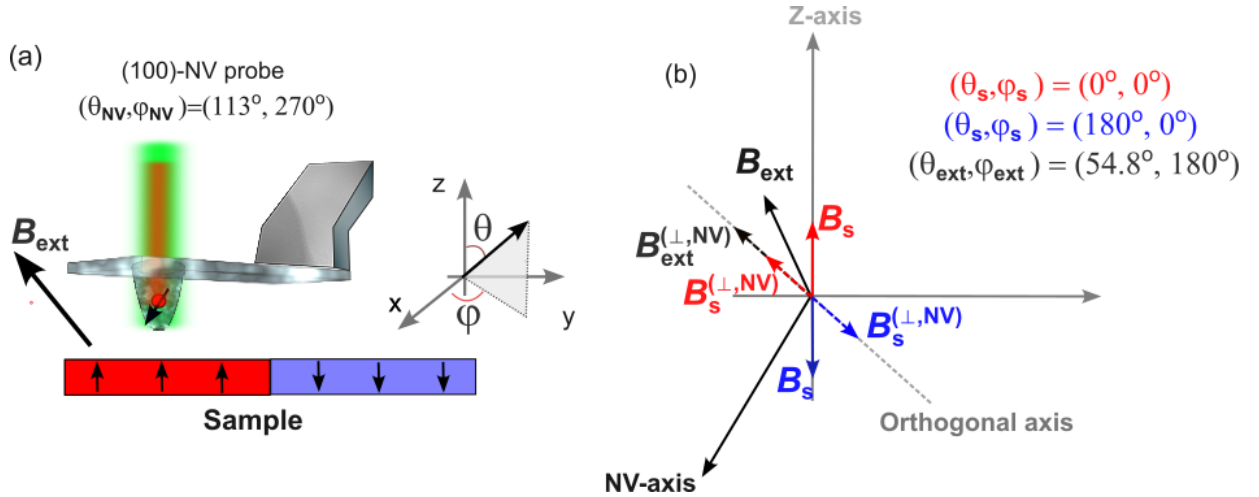

Figure S5: **Magnetic field components perpendicular to the NV-axis.** (a) schematic illustration of the (100)-NV tip scanning domains with magnetic moments pointing up and down. (b) Projection of the field components along the NV-axis.

During the acquisition of NV-PL quenching images in the presence of an off-axis field, the sensor will experience a total field with contributions from both the sample stray field and the field applied externally. Each contribution is described by the vector:

$$\vec{B}_i = B_i \langle \sin \theta_i \sin \varphi_i, \sin \theta_i \cos \varphi_i, \cos \theta_i \rangle \quad (3)$$

with  $i = s, \text{ext}$ , for the sample and external field, respectively. The parallel and perpendicular projections on the NV-axis are given by

$$B_i^{(\parallel, \text{NV})} = \vec{B}_i \cdot \hat{e}_{\text{NV}}, \text{ and } B_i^{(\perp, \text{NV})} = \left\| \vec{B}_i - \vec{B}_i^{(\parallel, \text{NV})} \right\| \quad (4)$$

As described in the main text, the quenching in the PL of the NV is mainly produced by spin-mixing effects induced by components of the field that are perpendicular to the NV-axis. Thus, the total field perpendicular to the NV-axis is given by the field compensation  $\mathbf{B}_{\text{total}}^{(\perp, \text{NV})} = \mathbf{B}_{\text{ext}}^{(\perp, \text{NV})} + \mathbf{B}_s^{(\perp, \text{NV})}$ . Table S1 summarizes the magnitude of the total OOP component of the field on domains with magnetization pointing up ( $\uparrow$ ) and down ( $\downarrow$ ), and the relative contrast between bright and dark areas in NV-PL images acquired at different values of the external applied field.

Table S1: Relative contrast between bright and dark areas in NV-PL quenching maps

| $B_{\text{ext}}$ [mT] | $B_{\text{total}\uparrow}^{(\perp, \text{NV})}$ [mT] | $B_{\text{total}\downarrow}^{(\perp, \text{NV})}$ [mT] | $C$ [%] |
|-----------------------|------------------------------------------------------|--------------------------------------------------------|---------|
| 0                     | 5                                                    | 5                                                      | 0       |
| 20                    | 24                                                   | 15                                                     | 23      |
| 25                    | 29                                                   | 20                                                     | 18      |
| 40                    | 44                                                   | 34                                                     | 13      |
| 60                    | 63                                                   | 54                                                     | 7       |

## Section 6: Additional NV-PL maps with the (100)-NV probe on a sample with $N=17$ , $X=7$ .

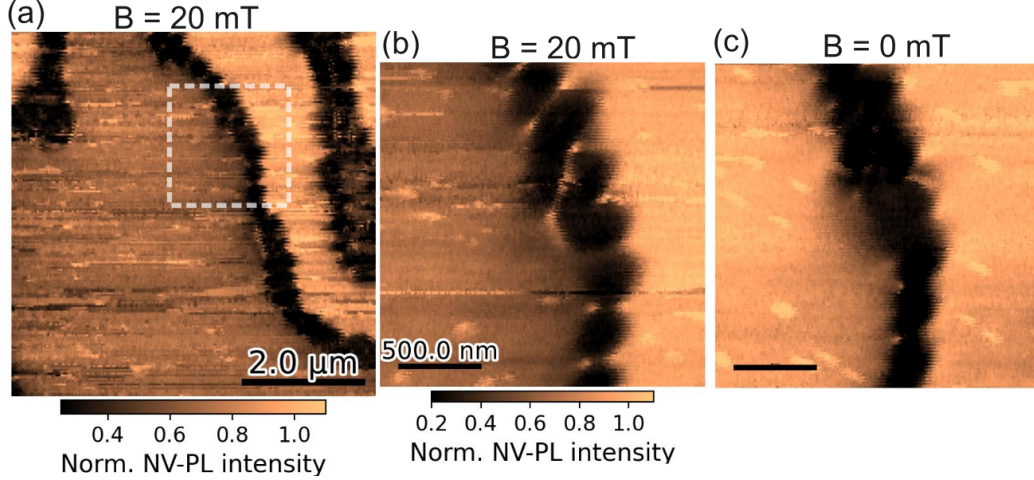

Figure S6: **NV-PL images with MFM-like contrast** . (a) NV-PL image of the sample  $[[\text{Co}(0.55\text{nm})/\text{Pt}(0.70\text{nm})]_6/\text{Co}(0.55\text{nm})/\text{Ru}(0.75\text{nm})]_{16}/[\text{Co}(0.55\text{nm})/\text{Pt}(0.70\text{nm})]_7$ , acquired with an external off-axis field of 20 mT. NV-PL images of the same area recorded (b) with and (c) without applying an off-axis field.

MFM-like contrast in NV-PL images is consistently observed when an off-axis field is applied to the NV during scanning. Figure S6 presents additional data acquired in a different sample. Figure S6(a) shows an NV-PL quenching images recorded on the sample  $[[\text{Co}(0.55\text{nm})/\text{Pt}(0.70\text{nm})]_6/\text{Co}(0.55\text{nm})/\text{Ru}(0.75\text{nm})]_{16}/[\text{Co}(0.55\text{nm})/\text{Pt}(0.70\text{nm})]_7$ , when applying an off-axis field of 20 mT in the direction  $(\theta_{\text{ext}}, \varphi_{\text{ext}}) = (54.8^\circ, 180^\circ)$ . There is strong quenching along the FM stripe, as well as a slight difference in the PL contrast between left and right AF domain. From Figures S6(b) and (c), it can be seen that the quenching along the FM stripe is uniform after turning the external field off, and the PL contrast at the AF domains is the same.

## Section 7: Additional ODMR measurements with the (111)-NV probe

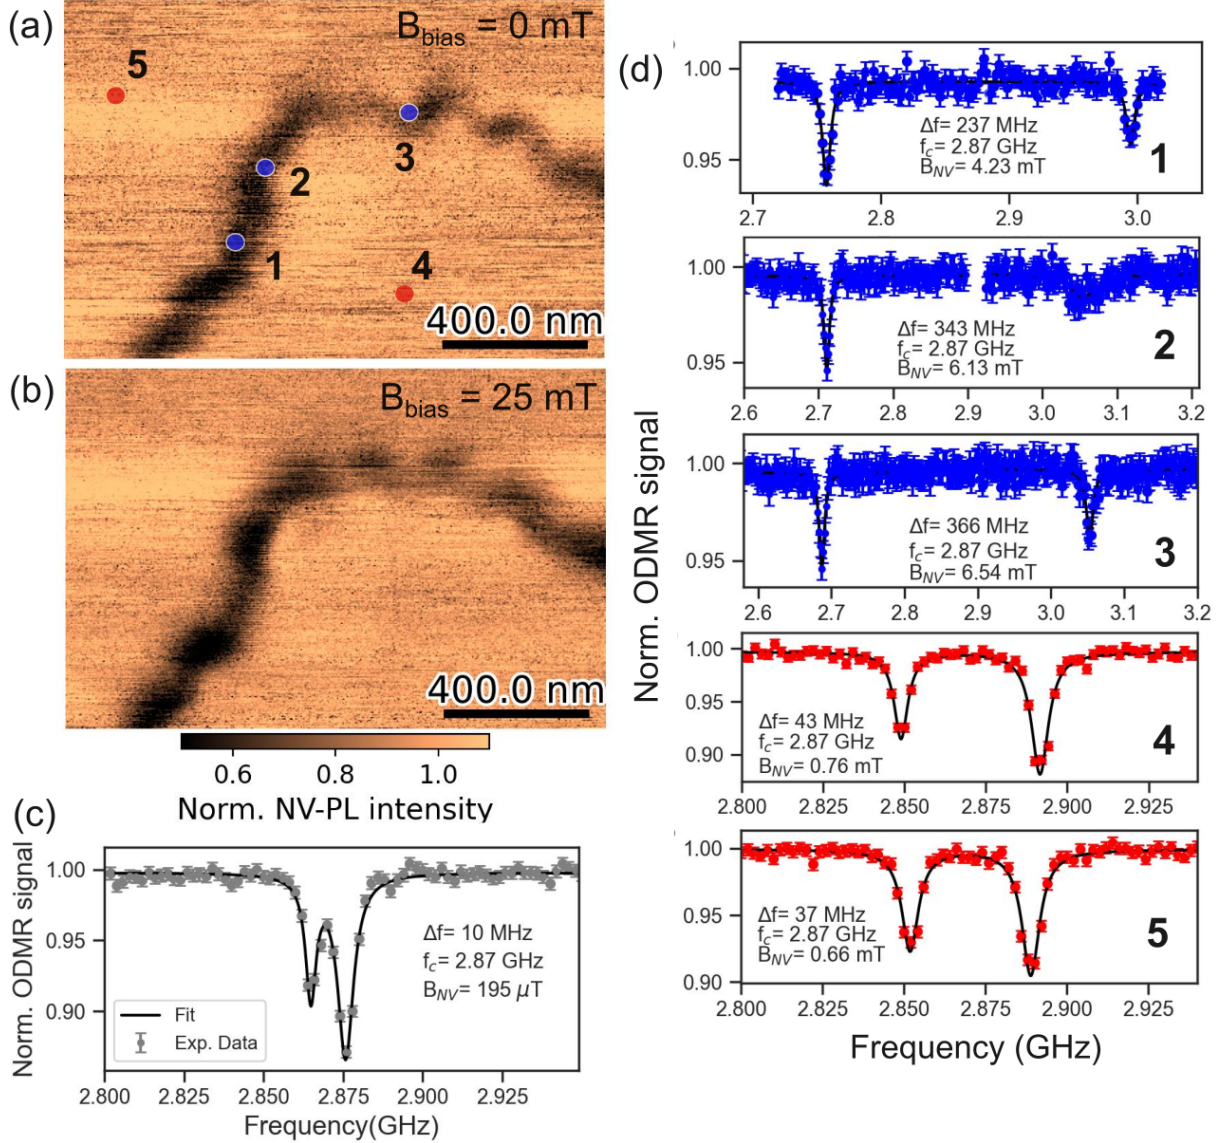

Figure S7: **Local ODMR measurements.** NV-PL quenching map (a) without and (b) with bias field along the NV-axis. (c) ODMR spectrum of the tip before approaching the sample. (d) ODMR spectra measured locally after approaching the sample and positioning the tip on the locations indicated in (a). The inset parameters in every plot correspond to the splitting ( $\Delta f$ ), the central frequency ( $f_c$ ), and the field sensed by the NV-center ( $B_{\text{NV}}$ ).

NV-PL quenching images recorded with the (111)-NV tip and acquired with and without an applied bias field are shown in Figure S7(a) and S7(b), respectively. The bias field, which is necessary for acquiring vector stray field maps, is applied along the NV axis. From the images, it is evident that the bias field does not significantly affect the NV-PL contrast. ODMR spectra acquired at the locations marked in Figure S7(a) indicate that, along the FM stripe, there is no significant magnetic field component perpendicular to the NV axis that could lead to spin mixing. Instead, we are primarily sensing the OOP field components that are aligned with the NV axis, which results in a symmetric Zeeman shift with respect to  $f_0=2.87$  GHz, as can be seen in Figure S7(d).

## **Section 8: Iso-B contours**

The acquisition of NV-PL images under MW excitation at a given frequency allows us to resolve iso-field contours, as can be observed in Figure S8. The images show contours of regions with a given stray field value together with the PL quenching along the FM stripe between AF domains. From the images, we can see the relative position of the different contours with respect to the FM stripe. Negative and positive values of the stray field are resolved by applying a bias field of 25 mT along the NV-axis. Pure iso-B images can be obtained when the NV-PL image acquired without MW excitation is subtracted. The dual iso-B images shown in the main text are obtained by taking the PL difference between two iso-B images.

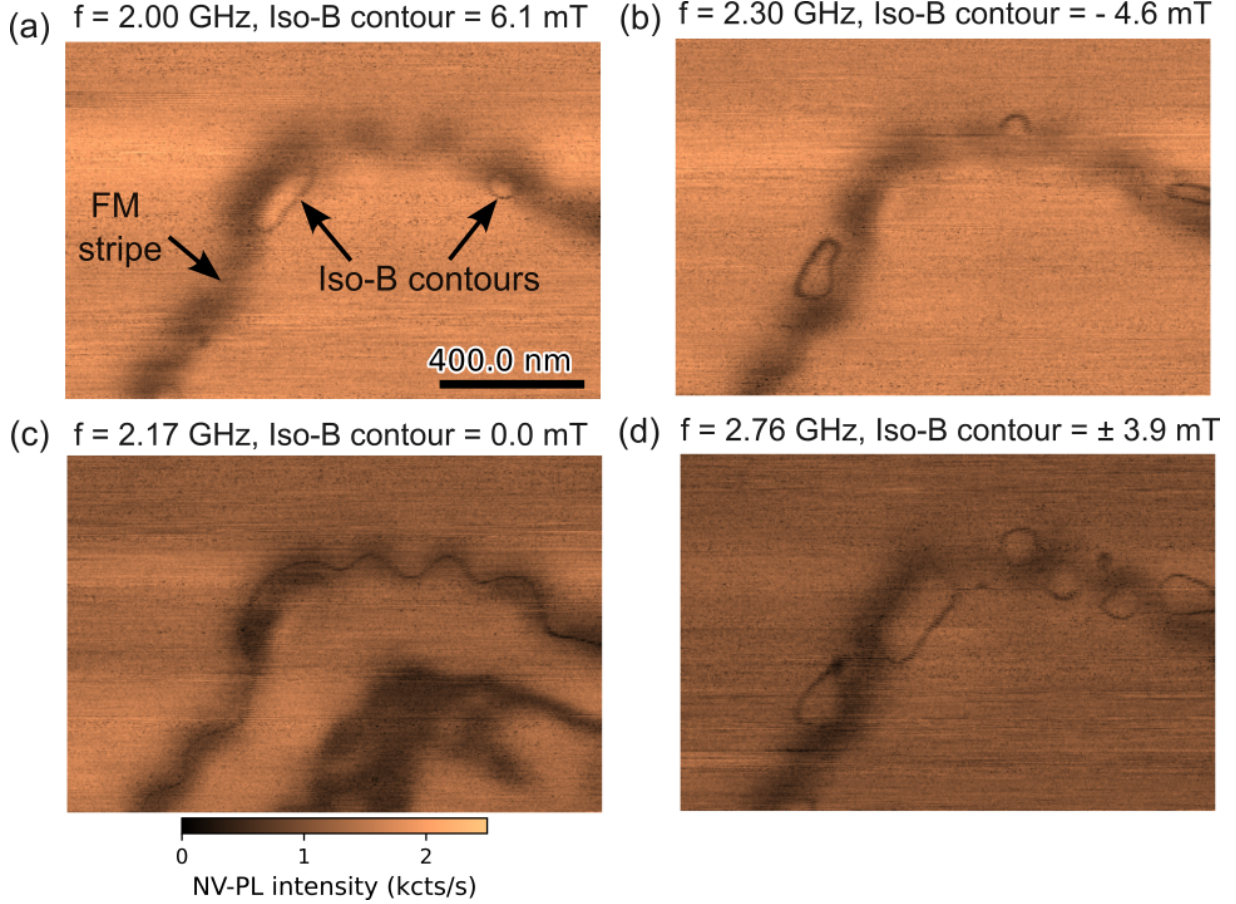

Figure S8: **Iso-B contours and NV-PL maps.** NV-PL images acquired while applying MW excitation to the NV at (a) 2.00 GHz, (b) 2.30 GHz, (c) 2.17 GHz, and (d) 2.76 GHz. A bias field of 25 mT was applied to record the images in (a)-(c), and 0 mT for the image in (d).

## Section 9: Reconstruction of the vector field components

In general, for static magnetic fields in source-free regions, the magnetic field components are not independent. Therefore, it is possible to derive all three field components above the sample surface at a given distance from the measurement of any single component.<sup>3,4</sup> By using Ampere's law and applying the reverse propagation method in Fourier space, we can obtain the field components  $(B_x, B_y, B_z)$ , at a constant  $d_{\text{NV}}$  using the measured  $B_{\text{NV}}$  projection, as given by:

$$B_x(k_x, k_y, d_{\text{NV}}) = -i \frac{k_x}{k} B_z(k_x, k_y, d_{\text{NV}}), \quad B_y(k_x, k_y, d_{\text{NV}}) = -i \frac{k_y}{k} B_z(k_x, k_y, d_{\text{NV}}), \quad (5)$$

with,

$$B_z(k_x, k_y, d_{\text{NV}}) = \frac{B_{\text{NV}}(k_x, k_y, d_{\text{NV}})}{n_z - i \frac{n_x k_x + n_y k_y}{k}}. \quad (6)$$

with  $\hat{e}_{\text{NV}} = \cos \varphi_{\text{NV}} \sin \theta_{\text{NV}} \hat{e}_x + \sin \varphi_{\text{NV}} \sin \theta_{\text{NV}} \hat{e}_y + \cos \theta_{\text{NV}} \hat{e}_z = n_x \hat{e}_x + n_y \hat{e}_y + n_z \hat{e}_z$  and  $k = \sqrt{k_x^2 + k_y^2}$ .  $\mathbf{k} = (k_x, k_y)$  is the wave-vector.

In section 2 we obtained  $\varphi_{\text{NV}} = 0^\circ$  and  $\theta_{\text{NV}} = 180^\circ$ . Therefore,  $n_x = n_y = 0$  and  $n_z = -1$ , and from the equation (6),  $B_z(k_x, k_y, d_{\text{NV}}) = -B_{\text{NV}}(k_x, k_y, d_{\text{NV}})$ . The IP stray field maps shown in Figure 4 of the main text were reconstructed after applying the inverse Fourier transform to the values obtained using the expressions in (5).

## section 10: Close-up view of the ODMR contrast on AF domains

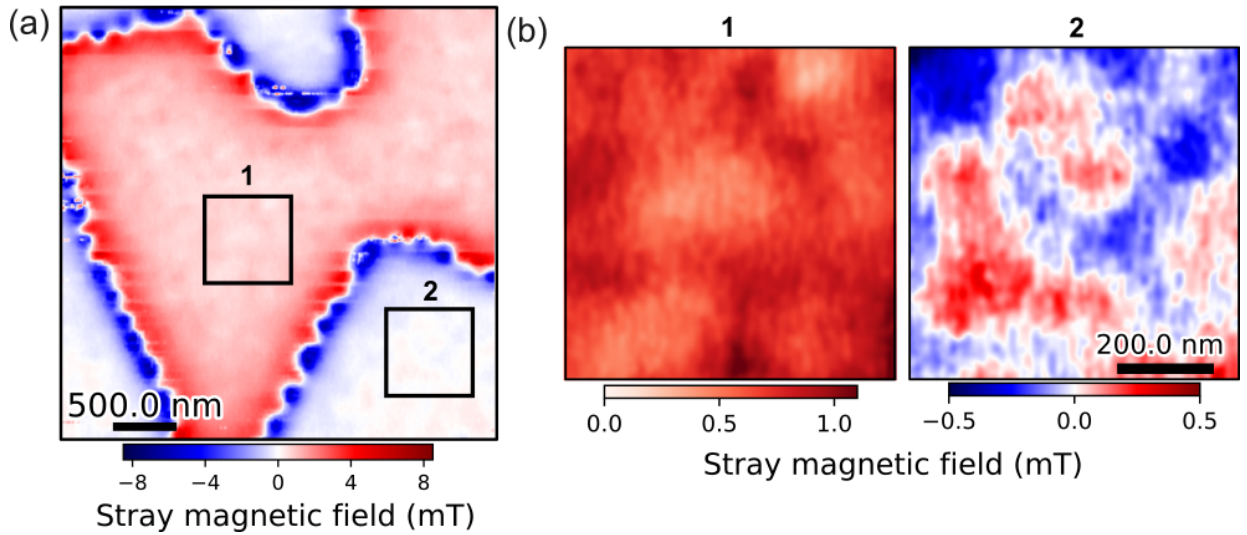

Figure S9: **ODMR contrast in the ROI.** (a) ODMR map shown in Figure 4(a) of the main text. (b) Close-up view in the ROI 1 and 2.

As described in the main text, a stray magnetic field of hundreds of  $\mu\text{T}$  up to around 1 mT is measured on the AF domains. In Figure S9, the close-up view of the region of interest (ROI) 1 and 2 in the ODMR map in Figure 4(a) in the main text show inhomogeneities of the stray field and thus imply the formation of small magnetization variations inside the AF domains. The observed variation of the stray field in the AF domains is most likely produced by uncompensated magnetization induced by local variation of the thin film thicknesses or due to granularity in the morphology of the sample surface. The morphology and granularity of the sample surface can be observed in the topography AFM images in Figure S10(a) and S10(b), acquired simultaneously with the MFM image shown in Figure S10(c).

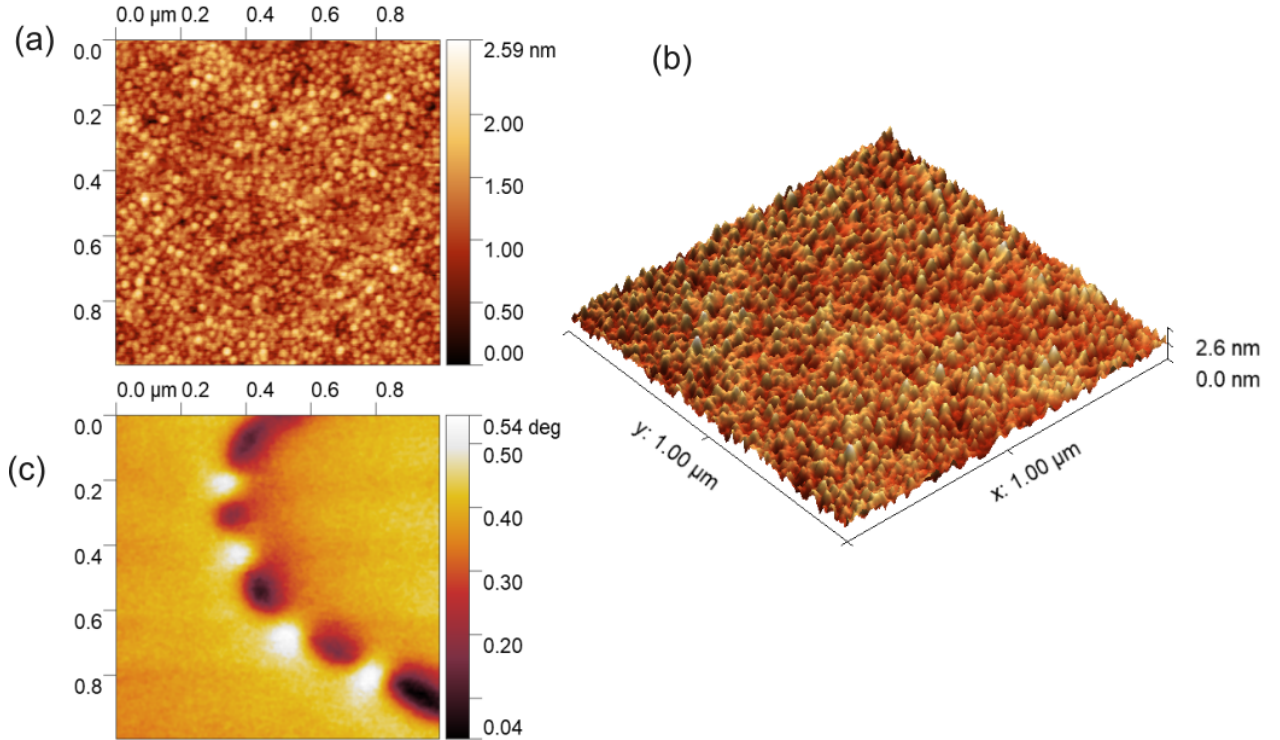

Figure S10: **Topography and MFM images.** (a)  $1\mu\text{m} \times 1\mu\text{m}$  2D and (b) 3D AFM topography image. (c)  $1\mu\text{m} \times 1\mu\text{m}$  MFM images.

## Section 11: OOP magnetization and DW shift

Figure S11(a) shows a 3D representation of the simulated structure with a square AF domain and sharp DW. The structure is modeled as four FM blocks with magnetization up and

down for AF coupling. The OOP magnetization of the FM blocks 1 and 3 is the same, and it is shown in the top image of Figure S11(b). The bottom image corresponds to the magnetization of blocks 2 and 4. To visualize the DW shift between the adjacent FM blocks, an overlap of the magnetization is shown in Figure S11(c). The DW shift at the position indicated by the white arrows in the top image in Figure S11(c) can be estimated by plotting the profile across the DW in the first and second FM block. The profiles are depicted in Figure S11(d), obtaining a lateral shift  $\delta \approx 40$  nm between DWs. This lateral shift is not uniform along the boundary of the AF domains, in some regions  $\delta$  can go down to 0 nm.

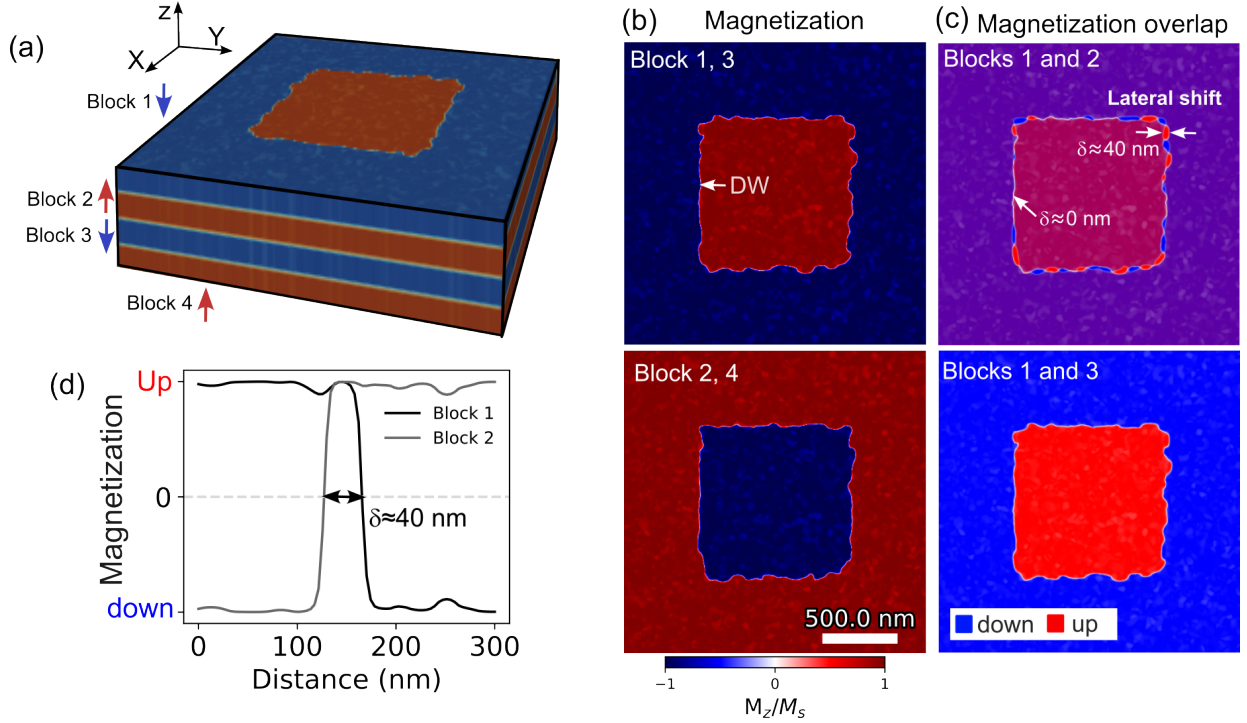

Figure S11: **DW-shift**. (a) Three-dimensional structure of the simulated square AF domain with sharp DW. (b) Top (bottom) image correspond to the OOP magnetization of the FM Blocks 1 and 3 (2 and 4). (c) OOP magnetization overlap of two different FM blocks to visualize the DW shift  $\delta$ . (d) Magnetization profile and DW shift between the FM blocks block 1 and 2 (3).

### Code for simulation of magnetization

```

/***** Interaction Energy Parameters *****/
A := 8.0e-12 //Heisenberg exchange [J/m]

```

```

Aex = A
A_IEC := -0.7e-3 // Interlayer exchange [J/m^2]
Ku1 = 0.6e6 // Uniaxial anisotropy downward [J/m3]
anisU = vector(0, 0, 1) // Direction of anisotropy axis
alpha = 0.01 // Gilbert damping
/***** Number of layers, GridSize, CellSize and geometry *****/
Lx := 2048e-9
Ly := 2048e-9
cyldiam := 1024e-9
dz := 0.75e-9 // Corresponds to the Ru layer
ithickness := 6.75e-9
N := 4 // Number of Co/Pt blocks (N-1 is the number of Ru layers)
X := 9 // Number of layers of thickness dz in a Co/Pt block
Nx := 512
Ny := 512
Nz := N*X + N - 1
Lz := Nz * dz
print("Nz=", Nz)
//Nz= 39
SetGridsize(Nx, Ny, Nz)
SetCellsize(Lx/Nx, Ly/Ny, dz)
SetPBC(8, 8, 0)
/***** Magnetic parameters of the sample *****/
Ms := 833e3 //Saturation magnetization [A/m]
Msat = Ms
ALL_layers := Layers(0, nz)
FM_layers := Layers(0, X)
for i := 1; i < N; i++ {
    FM_layers = FM_layers.add(Layers(i*(X+1), (i+1)*(X+1)-1))
}

```

```

}

setGeom(FM_layers)

IEC_layers_up := Layer(X + 1)
for i := 1; i < N-1; i++ {
  IEC_layers_up = IEC_layers_up.add(Layer(X + 1 + i*(X+1)))
}

IEC_layers_dn := Layer(X - 1)
for i := 1; i < N-1; i++ {
  IEC_layers_dn = IEC_layers_dn.add(Layer(X - 1 + i*(X+1)))
}

pf := Const((A_IEC) / (dz * Ms))
up := Masked(Shifted(m, 0, 0, 2), IEC_layers_up)
dn := Masked(Shifted(m, 0, 0, -2), IEC_layers_dn)
Bc := Mul(pf, Add(up, dn))
AddFieldTerm(Bc)
AddEdensTerm(Mul(Const(-0.5), Dot(Bc, M_full)))

r0 := cuboid(cyldiam, cyldiam, X*dz).transl(0, 0, -Lz/2+X*dz/2)
a0 := cuboid(Lx, Ly, X*dz).transl(0, 0, -Lz/2+X*dz/2).sub(r0)
r1 := r0.transl(0, 0, (X+1)*dz)
a1 := a0.transl(0, 0, (X+1)*dz)
r2 := r1.transl(0, 0, (X+1)*dz)
a2 := a1.transl(0, 0, (X+1)*dz)
r3 := r2.transl(0, 0, (X+1)*dz)
a3 := a2.transl(0, 0, (X+1)*dz)
m.SetInShape(a0, Uniform(0, 0, 1))
m.SetInShape(r1, Uniform(0, 0, 1))
m.SetInShape(a2, Uniform(0, 0, 1))
m.SetInShape(r3, Uniform(0, 0, 1))

```

```

m.SetInShape(r0, Uniform(0, 0, -1))
m.SetInShape(a1, Uniform(0, 0, -1))
m.SetInShape(r2, Uniform(0, 0, -1))
m.SetInShape(a3, Uniform(0, 0, -1))

grainSize := 32e-9
randomSeed := 7913279
maxRegion := 256
ext_makegrains(grainSize, maxRegion, randomSeed)
randSeed(randomSeed)
theta_max := 20.0
for i := 0; i < maxRegion; i++ {
    theta := theta_max / 3 * randNorm()
    theta = theta / 180 * pi
    phi := PI * rand()
    vu := vector(sin(theta)*cos(phi), sin(theta)*sin(phi), cos(theta))
    anisU.SetRegion(i, vu)
}

B := 0.001    // slight 1 mT offset field to facilitate the relaxation and minimization
Theta := 0.5
Theta = Theta / 180 * pi
Phi := 0.5
Phi = Phi / 180 * pi
MinimizerStop = 1e-6
TableAddVar(m.Average().Dot(vector(sin(Theta)*cos(Phi), sin(Theta)*sin(Phi), cos(Theta))), "<M>",
"none")
TableAdd(Edens_total)
B_ext = vector(B*sin(Theta)*cos(Phi), B*sin(Theta)*sin(Phi), B*cos(Theta))
TableAdd(B_ext)
TableAddVar(B, "Bext", "T")

```

```

relax()

saveas(m, "relaxed.ovf")

minimize()

saveas(m, "minimized.ovf") // this relaxed and subsequently minimized state is the one we use

```

## Code for simulation of stray field maps

To simulate the stray field from the magnetic state obtained from the previous code, we defined a larger simulation domain (larger Nz), loaded the magnetic state with the `m.loadfile` command, and fitted it into the simulation domain with the `m.getcell` and `m.setcell` commands. Finally, the field is calculated

```

A := 8.0e-12
Aex = A
A_IEC := -0.7e-3
Ku1 = 0.6e6
anisU = vector(0, 0, 1)
alpha = 0.01
Lx := 2048e-9
Ly := 2048e-9
cyldiam := 1024e-9
dz := 0.75e-9
ithickness := 6.75e-9
N := 4
X := 9
Nx := 512
Ny := 512
Nz := N*X + N - 1 + 100
nzlayers := N*X + N - 1
totalt := Nz * dz

```

```

thickness := 100 * dz

Lz := Nz * dz

print("Nz=", Nz)

//Nz= 139

SetGridsize(Nx, Ny, Nz)

SetCellsize(Lx/Nx, Ly/Ny, dz)

SetPBC(8, 8, 0)

//resizing...

Ms := 833e3

Msat = Ms

m.loadfile("N4X6-strayfield.out/minimized.ovf")

for i := 0; i < Nx; i += 1 {
  for j := 0; j < Ny; j += 1 {
    a := m.getcell(i, j, 0)
    b := m.getcell(i, j, 45)
    c := m.getcell(i, j, 90)
    d := m.getcell(i, j, 135)
    m.setcell(i, j, 0, a)
    m.setcell(i, j, 1, a)
    m.setcell(i, j, 2, a)
    m.setcell(i, j, 3, a)
    m.setcell(i, j, 4, a)
    m.setcell(i, j, 5, a)
    m.setcell(i, j, 6, a)
    m.setcell(i, j, 7, a)
    m.setcell(i, j, 8, a)
    m.setcell(i, j, 10, b)
    m.setcell(i, j, 11, b)
    m.setcell(i, j, 12, b)
  }
}

```

```

    m.setcell(i, j, 13, b)
    m.setcell(i, j, 14, b)
    m.setcell(i, j, 15, b)
    m.setcell(i, j, 16, b)
    m.setcell(i, j, 17, b)
    m.setcell(i, j, 18, b)
    m.setcell(i, j, 20, c)
    m.setcell(i, j, 21, c)
    m.setcell(i, j, 22, c)
    m.setcell(i, j, 23, c)
    m.setcell(i, j, 24, c)
    m.setcell(i, j, 25, c)
    m.setcell(i, j, 26, c)
    m.setcell(i, j, 27, c)
    m.setcell(i, j, 28, c)
    m.setcell(i, j, 30, d)
    m.setcell(i, j, 31, d)
    m.setcell(i, j, 32, d)
    m.setcell(i, j, 33, d)
    m.setcell(i, j, 34, d)
    m.setcell(i, j, 35, d)
    m.setcell(i, j, 36, d)
    m.setcell(i, j, 37, d)
    m.setcell(i, j, 38, d)
  }
}

ALL_layers := Layers(0, nzlayers)
FM_layers := Layers(0, X)
for i := 1; i < N; i++ {

```

```

FM_layers = FM_layers.add(Layers(i*(X+1), (i+1)*(X+1)-1))
}

setGeom(FM_layers)

saveas(B_demag, "B_demag_all")

```

## **Section 12: $T_1$ measurement with different NV-probes**

Figure S12 show local  $T_1$  measurements performed with different scanning diamond probes and represented in Figure 5 in the main text.

## **Section 13: NV-PL quenching contrast and laser power**

The quenching observed in the NV-PL maps acquired with the (111)-NV probe is produced by magnetic noise. The perpendicular components of the noise that are resonant with the NV transition affect  $T_1$  and reduce the PL intensity, as can be seen in Figure S12. There is a competition between the optical pumping from the excitation power of the green laser and the spin relaxation.<sup>5</sup> That means that the contrast in the NV-PL maps should be affected by the excitation power. Figure S13 shows a saturation curve measured on the (111)-NV tip with the sample engaged, from which we obtain a saturation power of 85  $\mu\text{W}$ . Additionally, NV-PL maps acquired in the same region with different excitation power are depicted in the figure. We can observe that there is not a significant change in the contrast of the NV-PL maps. This could be due to the fact that, in contrast to what has been observed in AF samples,<sup>5</sup> the field produced on the FM cores around the DWs could affect the competition between the optical pumping and the spin relaxation process.

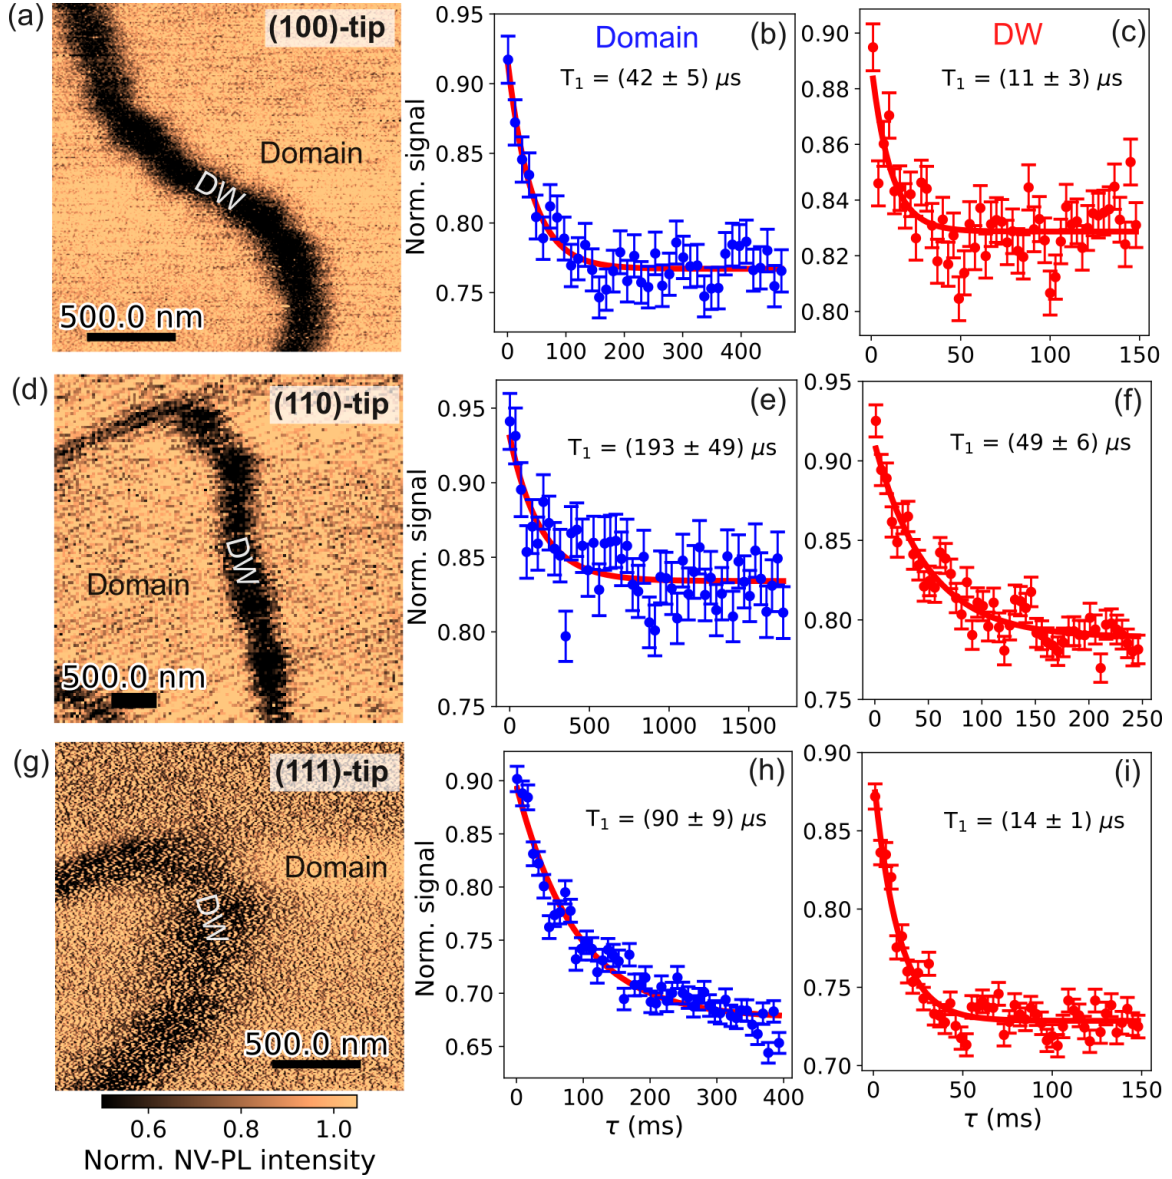

Figure S12: **Local  $T_1$  measurements.** NV-PL quenching map, and  $T_1$  measurement on a domain and a DW, acquired with (a)-(c) a (100)-NV tip, (d)-(f) a (110)-NV tip, and (g)-(i) a (111)-NV tip.

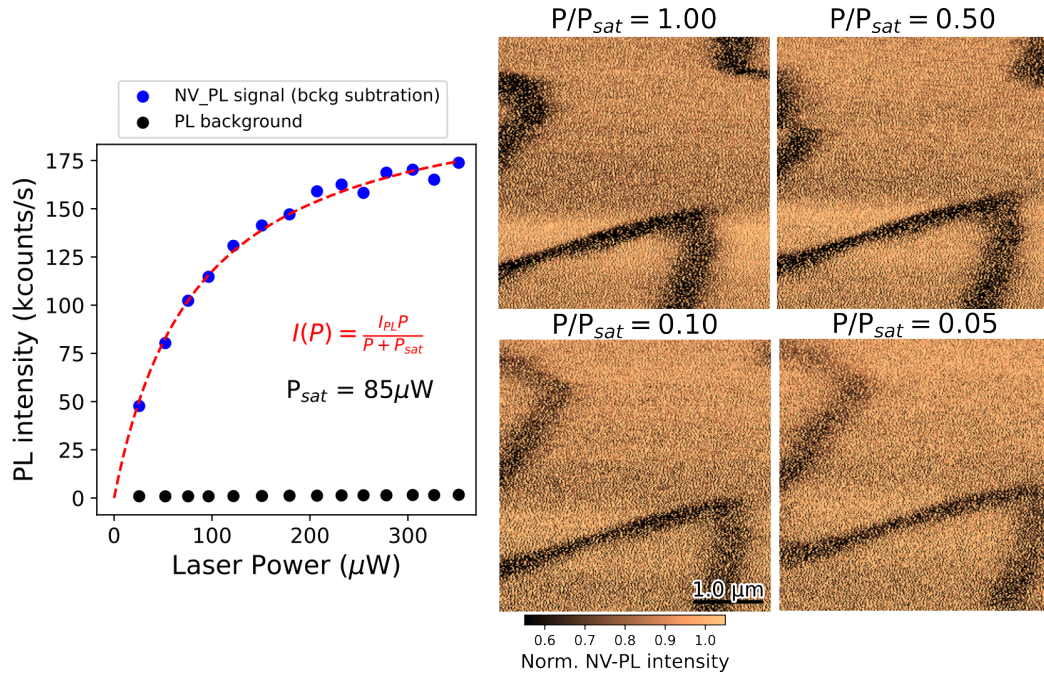

Figure S13: **NV-PL quenching contrast vs laser power.** Saturation curve measured on the (111)-diamond probe and NV-PL quenching images recorder with different excitation power below saturation.

## References

- (1) Hingant, T.; Tetienne, J.-P.; Martínez, L. J.; Garcia, K.; Ravelosona, D.; Roch, J.-F.; Jacques, V. Measuring the Magnetic Moment Density in Patterned Ultrathin Ferromagnets with Submicrometer Resolution. *Phys. Rev. Appl.* **2015**, *4*, 014003.
- (2) Hellwig, O.; Berger, A.; Fullerton, E. E. Domain Walls in Antiferromagnetically Coupled Multilayer Films. *Phys. Rev. Lett.* **2003**, *91*, 197203.
- (3) Lima, E. A.; Weiss, B. P. Obtaining vector magnetic field maps from single-component measurements of geological samples. *Journal of Geophysical Research: Solid Earth* **2009**, *114*.
- (4) Dovzhenko, Y.; Casola, F.; Schlotter, S.; Zhou, T. X.; Büttner, F.; Walsworth, R. L.; Beach, G. S.; Yacoby, A. Magnetostatic twists in room-temperature skyrmions explored

by nitrogen-vacancy center spin texture reconstruction. *Nature communications* **2018**, *9*, 2712.

- (5) Finco, A. et al. Imaging non-collinear antiferromagnetic textures via single spin relaxometry. *Nat. Commun.* **2021**, *12*, 767.
